# Supplementary material for: How to Promote Autonomous Driving with Evolving Technology: Business Strategy and Pricing Decision
Source: arXiv:2503.17174 source file (2025-03-21)
Supplement: Supplementary file 1 [file proposition4_analysis.tex]

We suggest that the influence of increasing initial software quality ($q$) on the consumer-abandon effect can be divided into three segments.

In the first segment, as $q$ increases, the proportion of consumers who delay their subscriptions under the $BS$ strategy gradually declines, thereby reducing the proportion of abandon-consumers and weakening the consumer-abandon effect.
However, as $q$ increases further, even if all consumers subscribe in Stage 1, there will still be at least $(1 - \alpha)$ of them (system-useless consumers) who abandon their subscriptions in Stage 2.
Consequently, under the $BS$ strategy, as $q$ increases, the proportion of abandon-consumers decreases and eventually converges to $1 - \alpha$ at the end of the first segment.

In the second segment, the proportion of abandon-consumers under the $BS$ strategy remains unchanged.
In contrast, under the $US$ strategy, the manufacturer can mitigate profit losses caused by abandon-consumers by shifting the software charge into the SSH charge.
This leads to an increase of consumer-abandon effect with $q$ in the second segment.

Ultimately, when the software fee is almost entirely transferred into the SSH charge under the $US$ strategy, the process enters the third stage.
In this segment, the $BS$ strategy maintains a fixed proportion of abandon-consumers as $1 - \alpha$, while the $US$ strategy essentially eliminates the profit losses associated with abandon-consumers.
Then, the consumer-abandon effect converges to a fixed, $\alpha$-determined upward trend as $q$ increases in the third segment.
A lower value of $\alpha$ leads to a higher number of abandon-consumers under the $BS$ strategy. Consequently, the profit loss that the $US$ strategy can avoid increases more rapidly with $q$, which leads to a higher increase rate of the consumer-abandon effect with $q$.

In summary, when the manufacturer adopts a subscription strategy, the consumer-abandon effect first weakens and then strengthens as $q$ increases, ultimately settling into a relatively stable upward trend determined by the size of $\alpha$. The smaller the value of $\alpha$, the stronger this final upward trend in the consumer-abandon effect as $q$ increases.
